# Supplementary material for: Approximability of Discriminators Implies Diversity in GANs
Source: arXiv:1806.10586 source file (2019-07-01)
Supplement: Supplementary file 1 [file appendix-experiment.tex]

\section{Details on experiment setups}
\label{appendix:experiment}

\paragraph{Setup}
Our data generating model $\mc{G}$ is the invertible
neural net generator (cf. Section~\ref{section:invertible-generator})
with identity covariance, i.e. $X=G_\theta(Z)$, where
$G_\theta:\R^d\to\R^d$ is a $\ell$-layer layer-wise invertible
feedforward net. We use the Leaky ReLU with negative slope 0.5 as the
activation function $\sigma$, whose derivative and inverse can be very
efficiently computed. The weight matrices of the layers are set to be
well-conditioned with singular values in between $0.5$ to $2$.

We choose the discriminator architecture according to the conjoined
discriminator design (Lemma~\ref{lemma:logp-neural-network}): an
inverse network with additional density computation branches. As
$\log\sigma^{-1'}$ is a piecewise constant function and cannot be
backproed, we instead model it as a trainable one-hidden-layer neural
network that maps reals to reals. We add constraints on all the
parameters in accordance with
Assumption~\ref{assumption:invertible-generator}.

\paragraph{Training}
To train both networks, we generate stochastic batches (with batch
size 64) from both the ground-truth generator and the trained
generator, and solve the min-max problem in the Wasserstein GAN
formulation with 5 discriminator steps in between each generator
step. We use the RMSProp optimizer~\cite{TielemanHi12} as our update
rule.

\paragraph{Evaluation metric} Our main evaluation metric will be the
neural net distance and the KL divergence. For the neural net
distance, we report once in a while a more optimized WGAN evaluation
loss in which the generator is held fixed and the discriminator is
trained from scratch to a (local) optimum. Note that this metric is
more representative than the training curve, as insufficient gradient
steps on the discriminator makes it of lower quality early in the
training. 

We also compute the KL divergence from the formula
\begin{equation*}
  \what{\dkl}(p^\star,p) = \E_{X\sim\what{p^\star}^n}[\log
  p^\star(X)-\log p(X)],
\end{equation*}
where $p^\star$ is the ground truth and $p$ is the current
generator. Note that the computability of the KL divergence is due to
that we have the formula of $\log p$ from the density formula, and as
the Wasserstein distance is not analytically computable, we regard the
KL divergence as a good criterion for distributional closedness. 

Our theory shows that for this conjoined choice of $\mc{G}$ and
$\mc{F}$ , the $\mc{F}$-distance reflects both the Wasserstein
distance and the KL divergence. We will test the hypothesis that WGAN
training works for minimizing KL, and the KL divergence and
$\mc{F}$-distance are reflective of each other.
